# Supplementary material for: Origin of the turn-on temperature behavior in WTe$_2$
Source: arXiv:1510.06976 source file (2015-11-04)
Supplement: Supplementary file 1 [file Supplemental_MIT_WTe2.pdf]

Supplemental Document

# Origin of the turn-on temperature behavior in $WTe_2$

Y. L. Wang[1,2], L. R. Thoutam[1, 3], Z. L. Xiao*[1, 3], J. Hu[4], S. Das[5], Z. Q. Mao[4], J. Wei[4], R. Divan[5], A. Luican-Mayer [5], G. W. Crabtree[1, 6], and W. K. Kwok[1]

[1] Materials Science Division, Argonne National Laboratory, Argonne, Illinois 60439, USA

[2] Department of Physics, University of Notre Dame, Notre Dame, Indiana 46556, USA

[3] Department of Physics, Northern Illinois University, DeKalb, Illinois 60115, USA

[4] Department of Physics and Engineering Physics, Tulane University, New Orleans, Louisiana 70118, USA

[5] Center for Nanoscale Materials, Argonne National Laboratory, Argonne, Illinois 60439, USA

[6] Departments of Physics, Electrical and Mechanical Engineering, University of Illinois at Chicago, Chicago, Illinois 60607, USA

**Derivation of MR ~ $(H/\rho_0)^2$ from the semiclassic two-band model:**

The two-band model, which in complex resistivity is given as:[15]

$$\rho = \frac{1+\mu_e\mu_h H^2 + i(\mu_h - \mu_e)H}{e[n_e\mu_e + n_h\mu_h + i(n_e - n_h)\mu_e\mu_h H]} \tag{S1}$$

The experimental resistivity $\rho_{xx}$ is given by the real part of equation (1). When $n_e = n_h = n$, the third term in the denominator varnishes and we get:

$$\rho_{xx}(T,H) = \rho_{xx}(T,0) + \rho_{xx}(T,0)\mu_e\mu_h H^2 \tag{S2}$$

with
$$\rho_{xx}(T,0) = [en(\mu_e+\mu_h)]^{-1} = [en\mu_e(1+\kappa)]^{-1} \tag{S3}$$

where $\kappa = \mu_h/\mu_e$. This leads to $\mu_e = [en(1+\kappa)\rho_{xx}(T,0)]^{-1}$ and $\mu_e\mu_h = \kappa\mu_e^2 = \kappa[en(1+\kappa)\rho_{xx}(T,0)]^{-2}$. By defining $\alpha = \kappa[ne(1+\kappa)]^{-2}$, we obtain MR = $\alpha(H/\rho_0)^2$

That is, Eq.1 (with m = 2) can be directly derived from the two-band model for the case of perfectly compensated charge carriers. The fact of $\alpha$ is a constant in our sample, indicates that both the density $n$ and mobility ratio $\kappa$ are temperature insensitive.

**Table SI. Parameters of the measured samples**

| Sample # | I | II |
|---|---|---|
| Thickness (μm) | 0.284 | 60 |
| Width (μm) | 5.66 | 560 |
| Separation of $V_{xx}$-leads (μm) | 3.76 | 700 |
| Separation of $V_{xy}$-leads (μm) | 3.80 | N/A |
| $\rho_{xx}$ at 4K (μΩcm) | 2.73 | 3.36 |
| m | 1.92 | 1.90 |
| $\alpha$ $(\mu\Omega cm/T)^m$ | 25 | 85 |

# FIG.S1

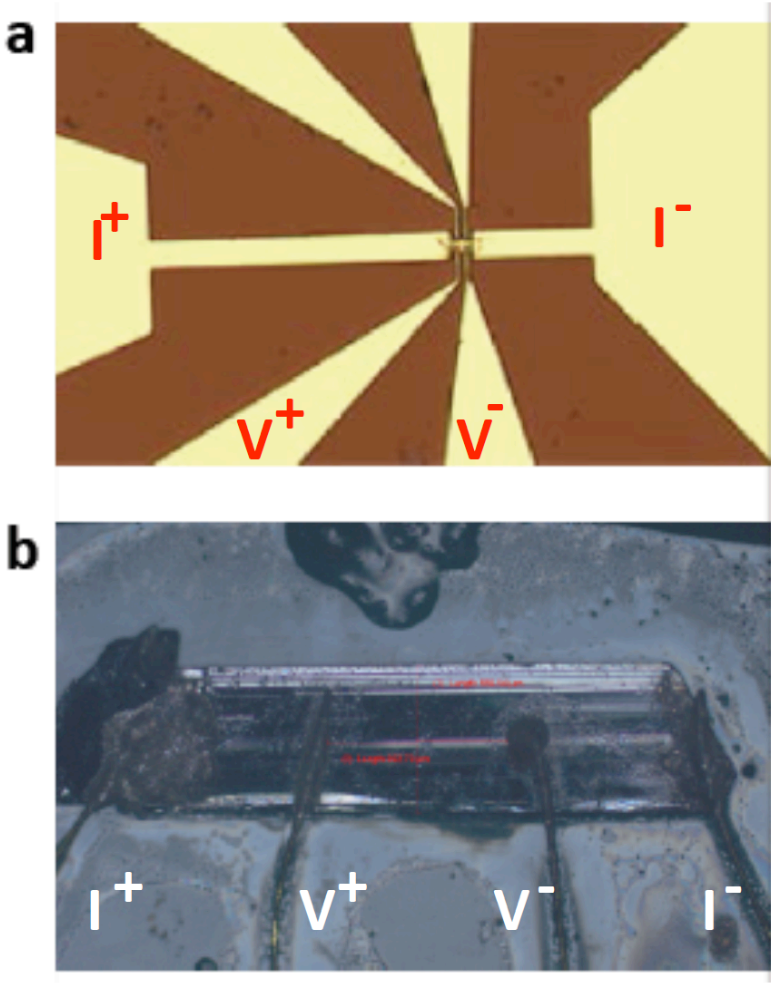


Optic images of sample I (a) and sample II (b). The electric contacts of sample II were made of silver paste. For sample I, we used photolithography followed by evaporation deposition of 300-500 nm thick Au layer with a 5 nm thick Ti adhesion layer to better define the contacts. The current flows along the a-axis (longitudinal direction in the image). The magnetic field is always perpendicular to the current (along the c-axis, perpendicular to the sample surface).

**FIG.S2**

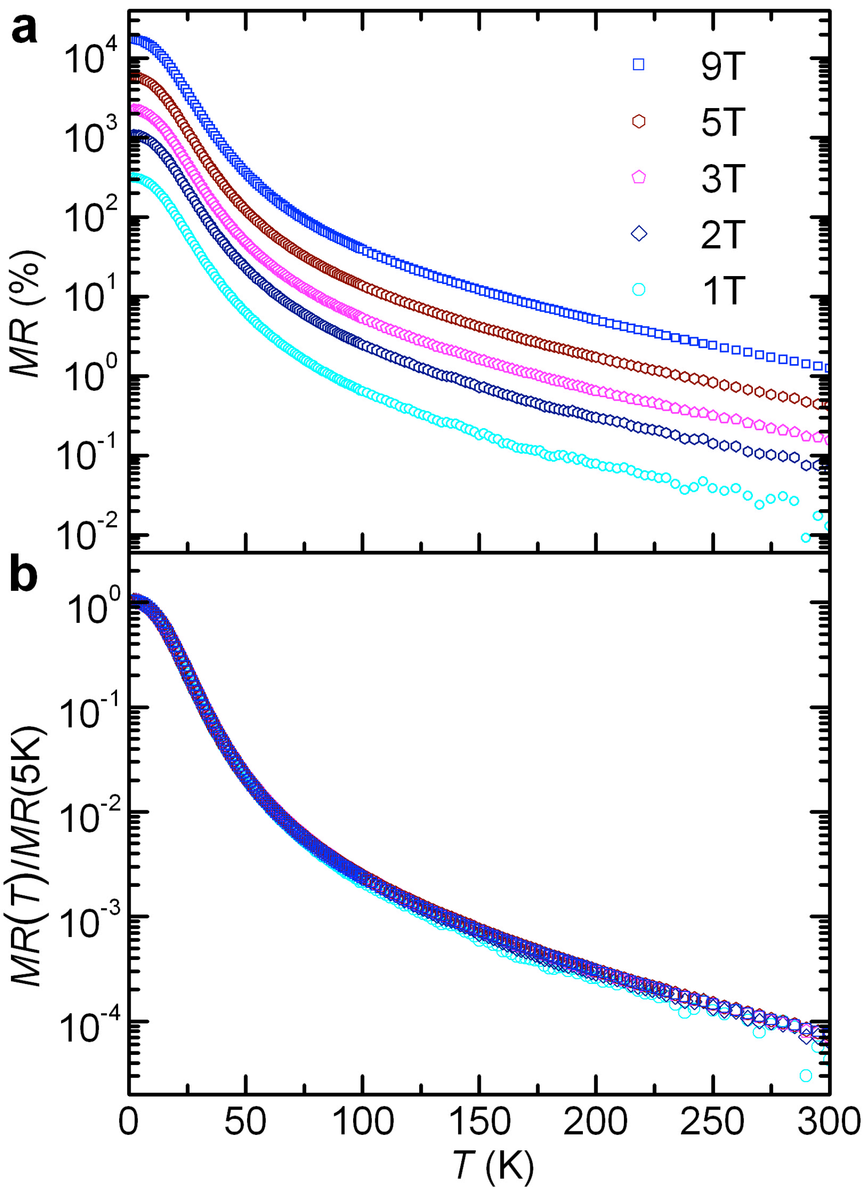


Temperature dependence of the magnetoresistances obtained at various fixed magnetic fields. (a) Original data, (b) Normalized with the values at 5K

# FIG.S3

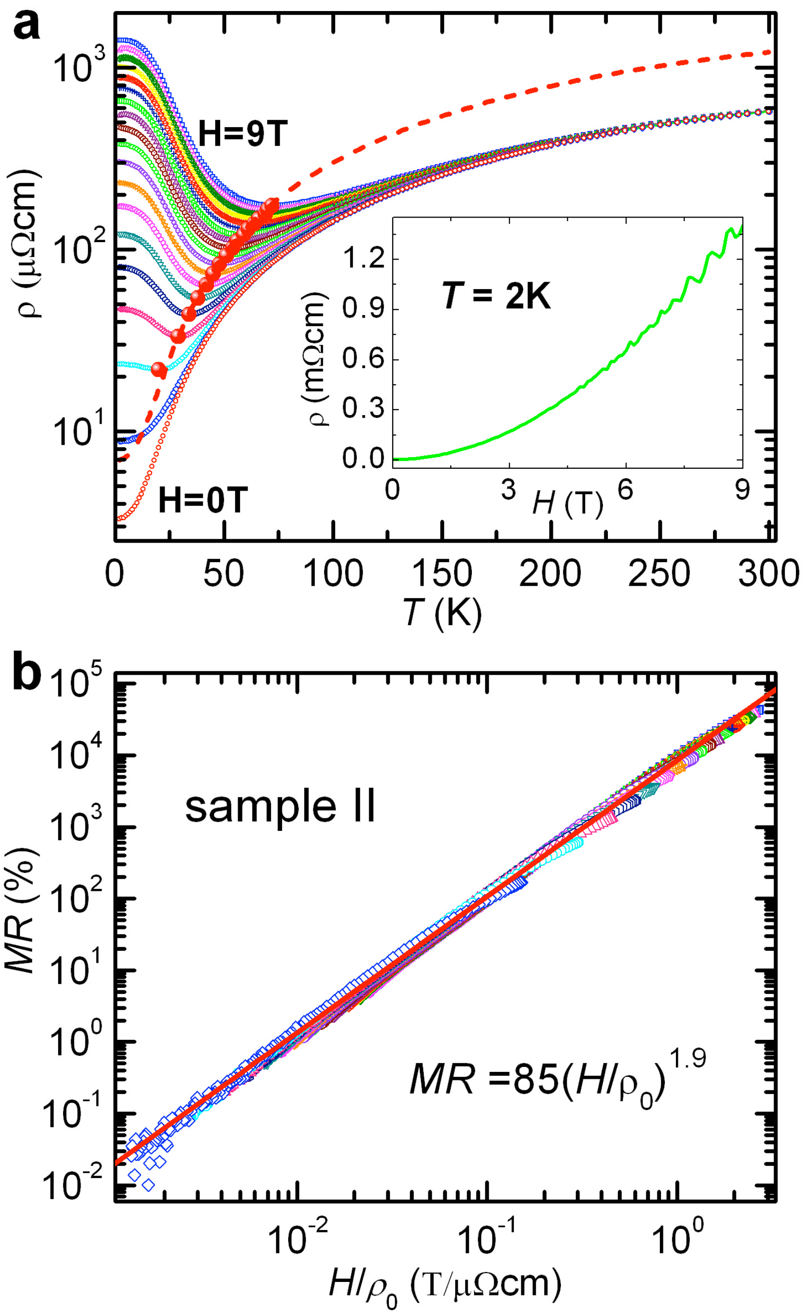


Kohler's rule scaling analysis of the temperature dependence of the magnetoresistances for sample II. (a) Original data. The magnetic field interval is 0.5 T. The inset shows the quantum oscillation in the *R*(*H*) curve at 2K, indicating the high quality of the crystal. (b) Kohler's rule scaling of the data in (a)

# FIG.S4

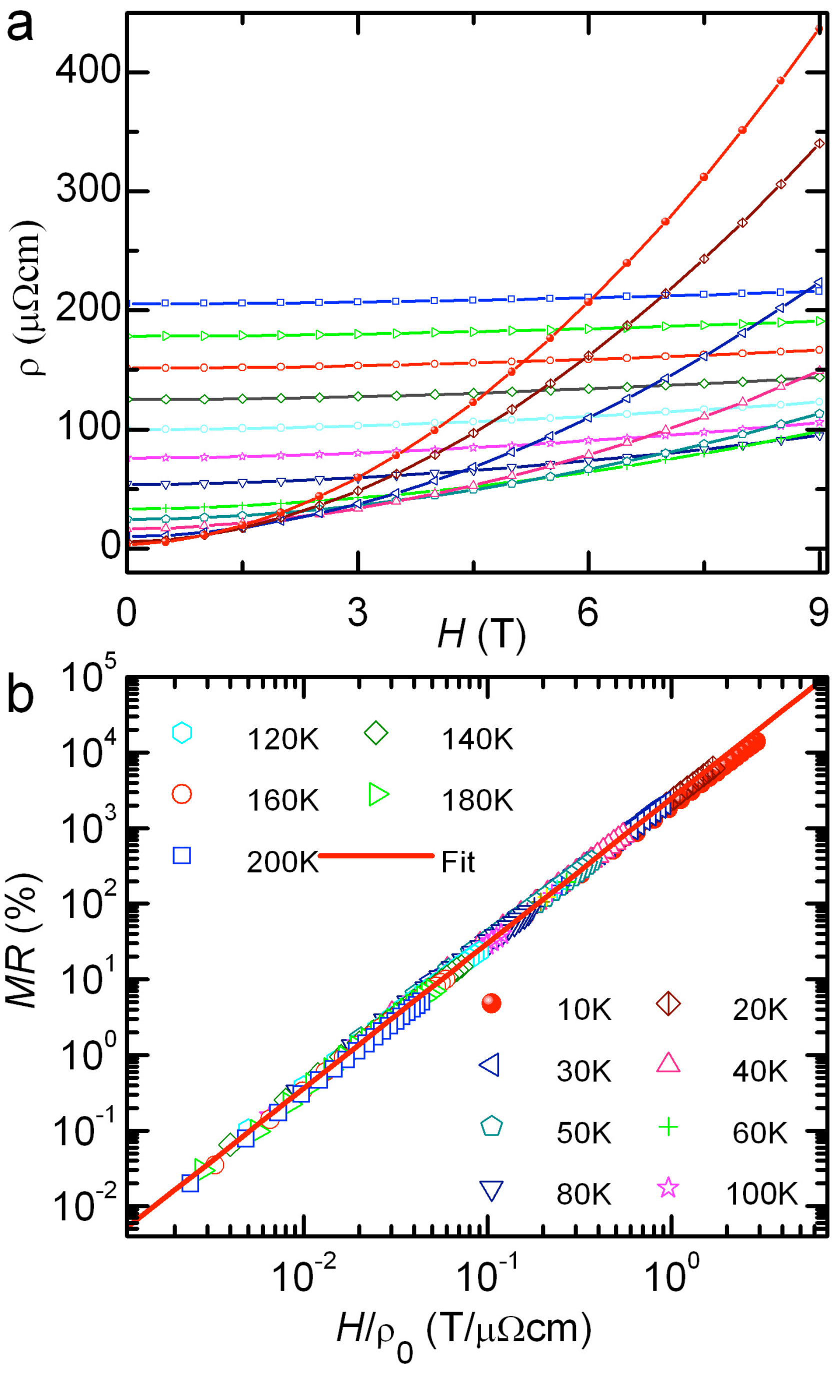


Kohler's rule scaling for the magnetic field dependence of the resistivity for sample I at various temperatures. (a) Original data, (b) Kohler's rule scaling. The symbols are the same in (a) and (b).

## FIG.S5

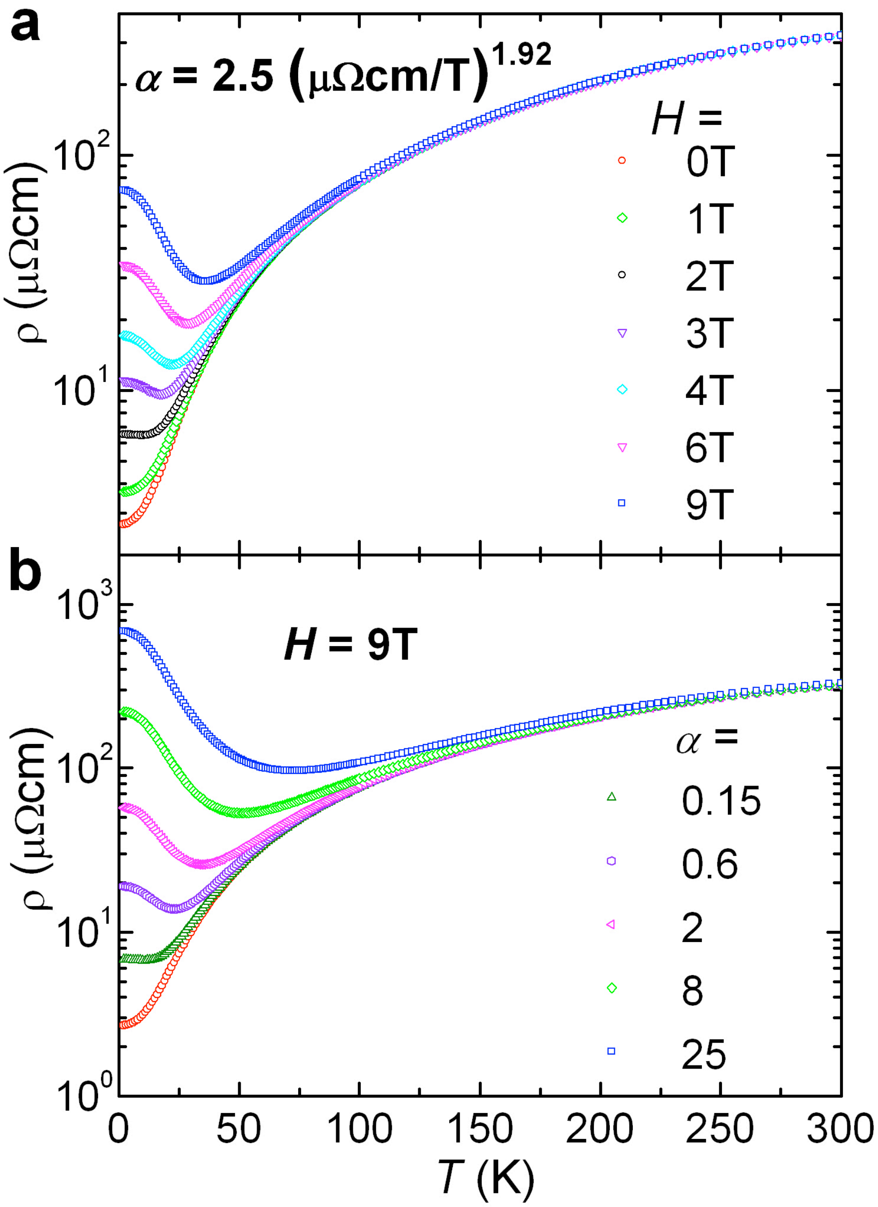


Effects of the value of *a* on the temperature behavior of the total resistivity. (a) At *a* = 2.5 (mWcm/T)$^{1.92}$ and various magnetic fields. (b) In 9 T and various $\alpha$.
